# Supplementary material for: Evaluating Robustness of Reward Models for Mathematical Reasoning
Source: arXiv:2410.01729 source file (2024-10-02)
Supplement: Supplementary file 1 [file appendix_bar_mrr.tex]

\begin{figure}[t!]
    \centering

    \includegraphics[width=0.72\textwidth]{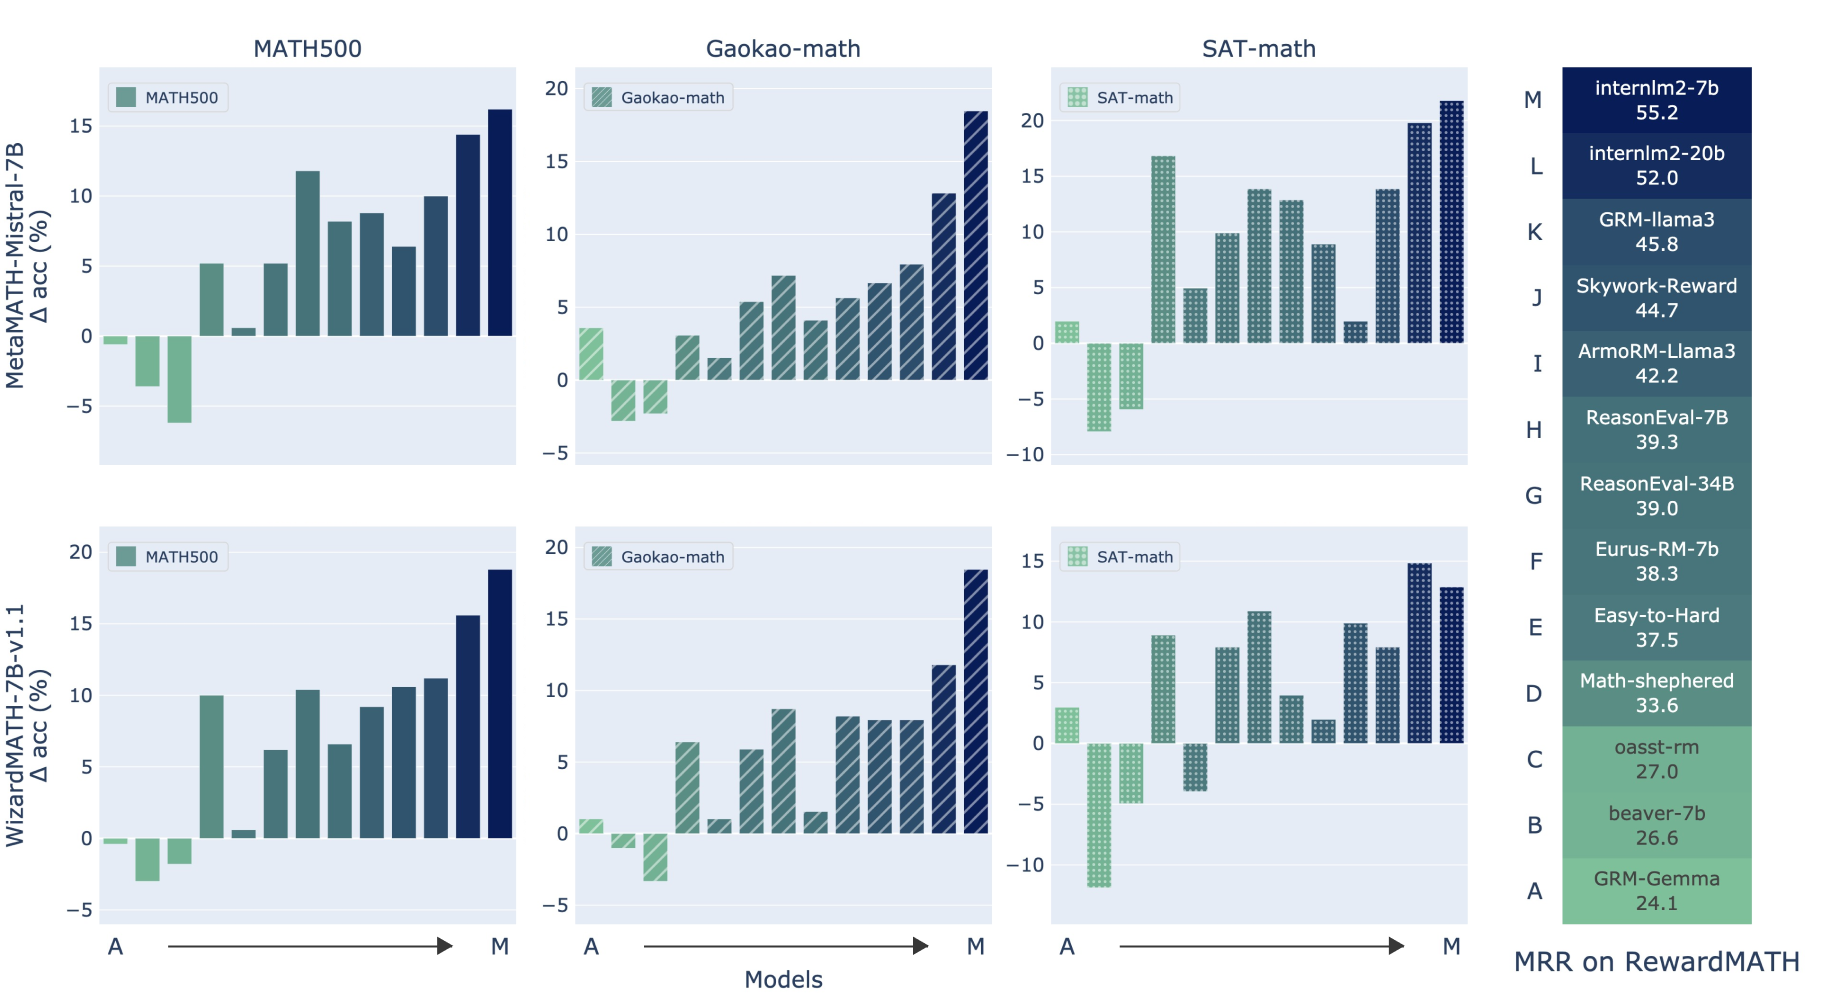}

    \caption{MRR on RewardMATH}
    \label{fig:appendix_bar_MRR}
\end{figure}
